# Supplementary material for: Detecting Contextual Anomalies by Discovering Consistent Spatial Regions
Source: arXiv:2501.08470 source file (2025-01-14)
Supplement: Supplementary file 1 [file X_supplementary.tex]

\clearpage
\setcounter{page}{1}
%%%%%%%%% TITLE - PLEASE UPDATE
% \title{Supplementary materials}
\maketitlesupplementary

%%%%%%%%% BODY TEXT
\section{Additional Experiment Results}
\noindent\textbf{Region proposal using semantic segmentation model.}
In the main paper, we compare our region proposal method with pre-trained off-the-shelf semantic segmentation model (SegFormer \cite{xie2021segformer}). The most direct way of utilizing segmentation model is to take its direct output (pixel level labels) as the regional map, we use the average output of all training data in StreetScene dataset from the pre-trained SegFormer to generate the region proposal. We also take a step further, utilize Gaussian mixture model to cluster the average logits to formulate the region map. Both region maps are shown in Fig.~\ref{fig:seg_region}. It is clear that, region map using the Gaussian mixture model shows a significant improvement in terms of region separation. The sidewalks and building are well separated. However, using segmentation model can not incorporate motion information into the region discovery, thus such region map can not support the detection of car/bike out of lane or wrong way anomalies. 
\begin{figure}
    \centering
    \includegraphics[width=1\linewidth]{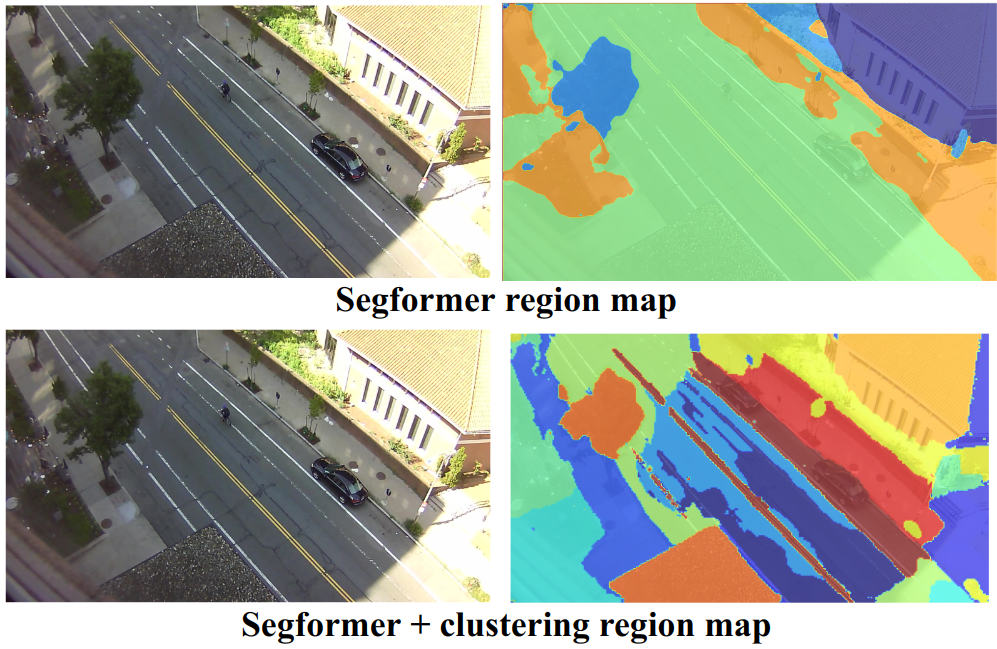}
    \caption{Region map generated from SegFormer \cite{xie2021segformer}. \textbf{Top}: region map using average logits \textbf{Bottom}: region map using GMM clustering  }
    \label{fig:seg_region}
\end{figure}

\noindent\textbf{Impact of LPIPS threshold.} By fixing the discovered region ($K =12$) and feature representation, we perform a parameter analysis of setting different $\alpha$ to filter out  
We explored the effect of the weight $\alpha$ that trades off the detection quality and anomaly detection performance, summarized in Figure \ref{fig:alpha_weight}. We can see that the algorithm clearly benefits from using LPIPS to remove irrelevant false detection. We achieved the best overall anomaly localization results (RBDC/TBDC) when $\alpha=0.25$.

\noindent\textbf{Impact of different clustering for region discovery.} Table \ref{tab:different_clustering} evaluates the performance using various distance or density-based clustering methods and Gaussian mixture models without full covariance.  In all cases, the performance significantly drops. It is critical to capture relationships between attribute channels (e.g., category+speed or category+direction) to discover high-quality meaningful regions. 

\begin{table}[htbp!]
    \centering
    \begin{tabular}{|c|c|c|c|}
    \hline
       \textbf{Methods} & \textbf{RBDC} & \textbf{TBDC} & \textbf{AUC}\\
      \hline
      K-means & 25.4 &46.3&\textbf{67.5}\\
      SLIC & 16.2 &57.3&60.1\\
       GMM + spherical cov. & 14.5 &56.2&53.8\\
       GMM + diagonal cov. & 16.6 &49.5&58.5\\
      GMM + tied cov. & 16.2 &56.7&62.4\\
        GMM + Spatial affinity & 28.9 &53.9&66.0\\
        GMM & \textbf{34.0} &\textbf{62.5}&67.0\\
      \hline
    \end{tabular}
    \caption{Performance using different clustering methods to discover regions. All experiments set $K =12$ and use same set of feature representation. }
    \label{tab:different_clustering}
\end{table}

% \begin{table}[ht]
% \centering
% \begin{tabular}{|c|c|c|}
% \hline
% \textbf{Column 1}                     & \textbf{Column 2} & \textbf{Column 3} \\ \hline
% \multirow{3}{*}{\rotatebox{90}{Rotated Text}} & Data 1 & Data 2 \\ \cline{2-3}
%                                        & Data 3 & Data 4 \\ \cline{2-3}
%                                        & Data 5 & Data 6 \\ \hline
% Regular 1                              & Data 7 & Data 8 \\ \hline
% Regular 2                              & Data 9 & Data 10 \\ \hline
% \end{tabular}
% \caption{Table with rotated multirow text sharing the first column with Data1}
% \end{table}
\begin{figure}
    \centering
    \includegraphics[width=1\linewidth]{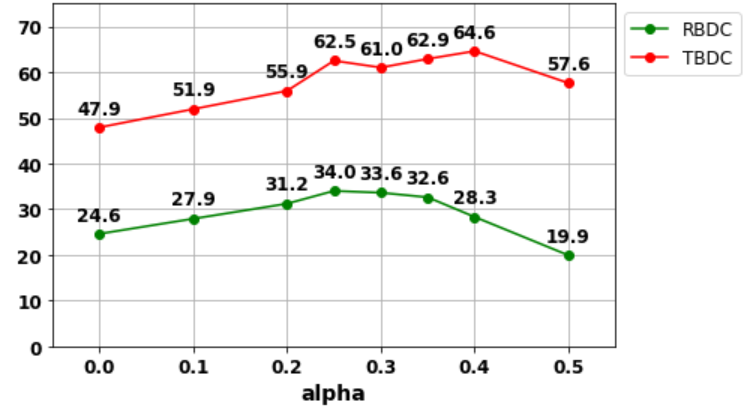}
    \caption{Sensitivity to the LPIPS threshold parameter $\alpha$ to filter false positive region detection.}
    \label{fig:alpha_weight}
\end{figure}

% Compared to training GMM with object class feature (4 dimensions in our case), training GMM with the CLIP feature $f_{app} \in \RR^{512}$ substantially increase the number of parameters need to be estimated. Parameters of covariance $\Sigma_i$ per mode increases from 16 to $262144$ but receive no performance improvement. 

\noindent\textbf{Detection performance in Street Scene} We note that the performance of any object-centric VAD method is upper-bounded by the number of objects it detects at the earliest stage.  Table \ref{tab:det_perf} reports the detection rates of objects and tracks for the Street Scene dataset.  In particular, due to lighting conditions, small objects, and occlusions, we found that solely depending on pre-trained object detection only captures 61.2\% of the total anomalous bounding boxes.  When combined with our background subtraction merging technique, 87.7\% of the bounding boxes can be covered. 

\begin{table}[htbp!]
    \centering
    \begin{tabular}{|c|c|c|}
    \hline
      \textbf{Detection Setting} &  \textbf{RBDR}&\textbf{TBDR} \\
       \hline
        % Ped2 & YOLOv5-x & 92.9 & 100.0\\
        
        % Avenue & YOLOv5-x & 86.6 & 71.7\\
        
        % ShanghaiTech & YOLOv5-x & 96.7 & 98.7 \\
    
        YOLOv8-x & 61.2 & 96.6 \\
    
        YOLOv8-x+ BG & 87.7 & 99.0\\
        \hline
    \end{tabular}
    \caption{Detection coverage in the Street Scene dataset. BG stands for background subtraction.}
    \label{tab:det_perf}
\end{table}
\noindent\textbf{A closer look at VAD performance in Street Scene.} We achieve SoTA performance in terms of video anomaly localization (RBDC) in Street Scene, we want to further investigate what types of anomalies that we did great and what types of anomalies we did not. Based on the description of anomaly types in \cite{ramachandra_street_2020}, we manually labelled the ground truth with additional anomaly types (17 types). We plot the RBDC/TBDC area under curve between false positive rate 0 to 1 for each type of anomalies shown in Fig.~\ref{fig:mainfig}. Our method capture most of the spatial-context dependent anomalies like jaywalkers, bikers out side the lane. Due to the compactness of our feature presentation, our method did not perform well on long term anomalies like loitering. The result further illustrates the strong spatial-context dependent anomaly detection ability of our proposed method. We will try to address long-term anomalies in our future research.
\begin{figure*}[!t]
\centering
    \begin{subfigure}[b]{1\textwidth}  % Width of the first figure
        \centering
        \includegraphics[width=\textwidth]{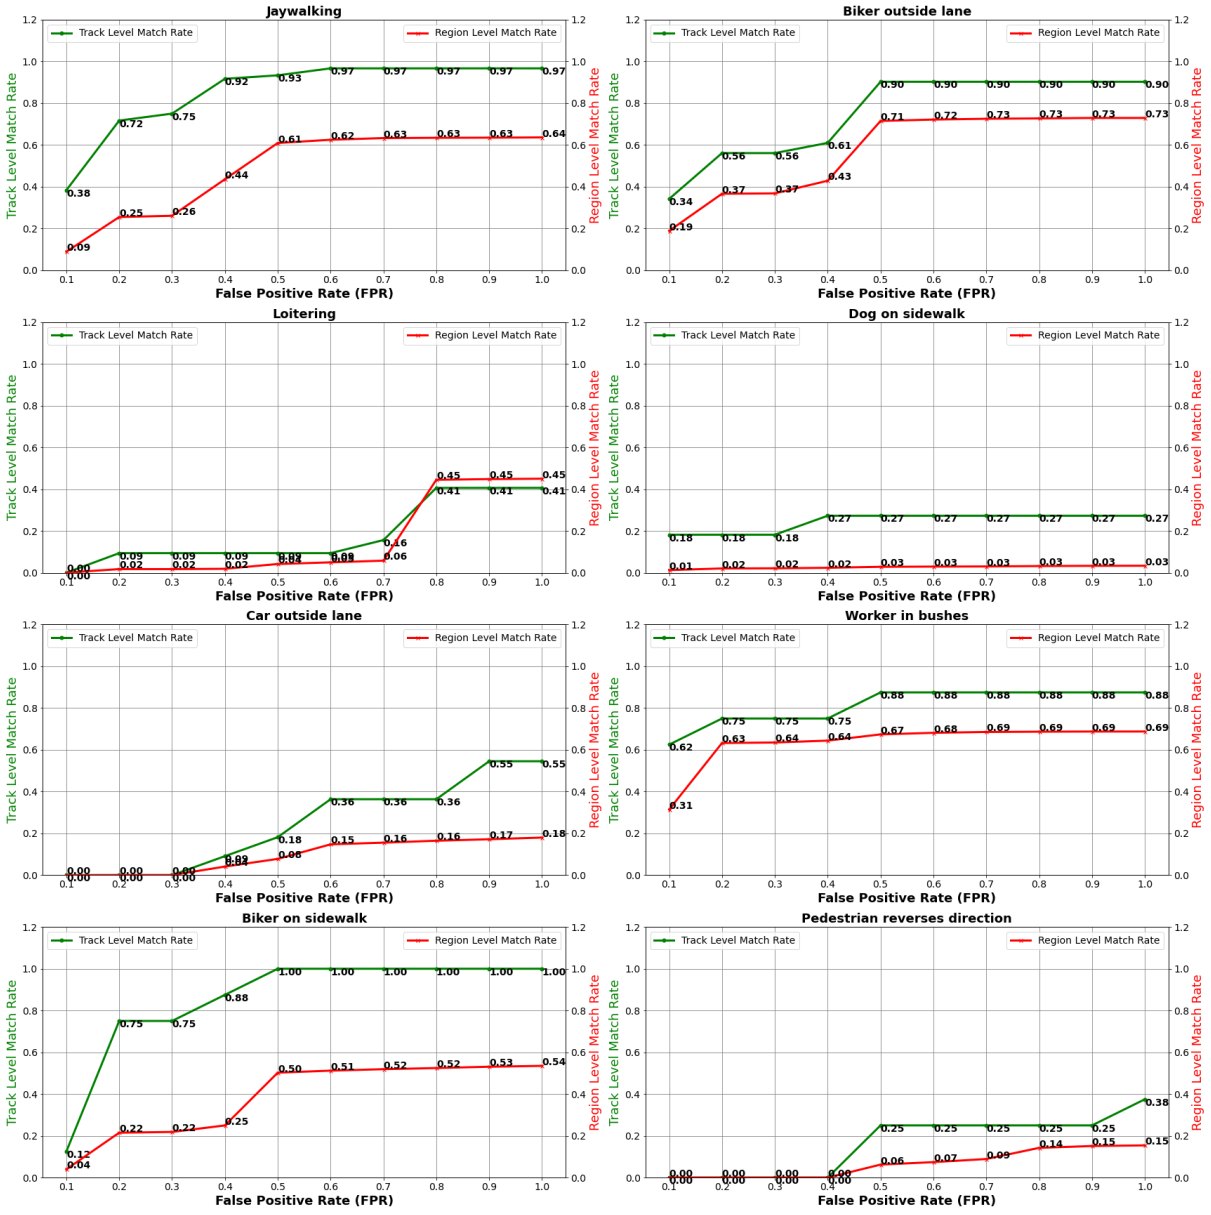}
        \label{fig:subfig1}
    \end{subfigure}
    \hfill
    
    \caption{Detailed RBDC/TBDC ROC curve of our method in Street Scene Dataset.  }
    \label{fig:mainfig}
\end{figure*}
\begin{figure*}
    \ContinuedFloat
    \centering
    \begin{subfigure}[b]{1\textwidth}  % Width of the second figure
        \centering
        \includegraphics[width=\textwidth]{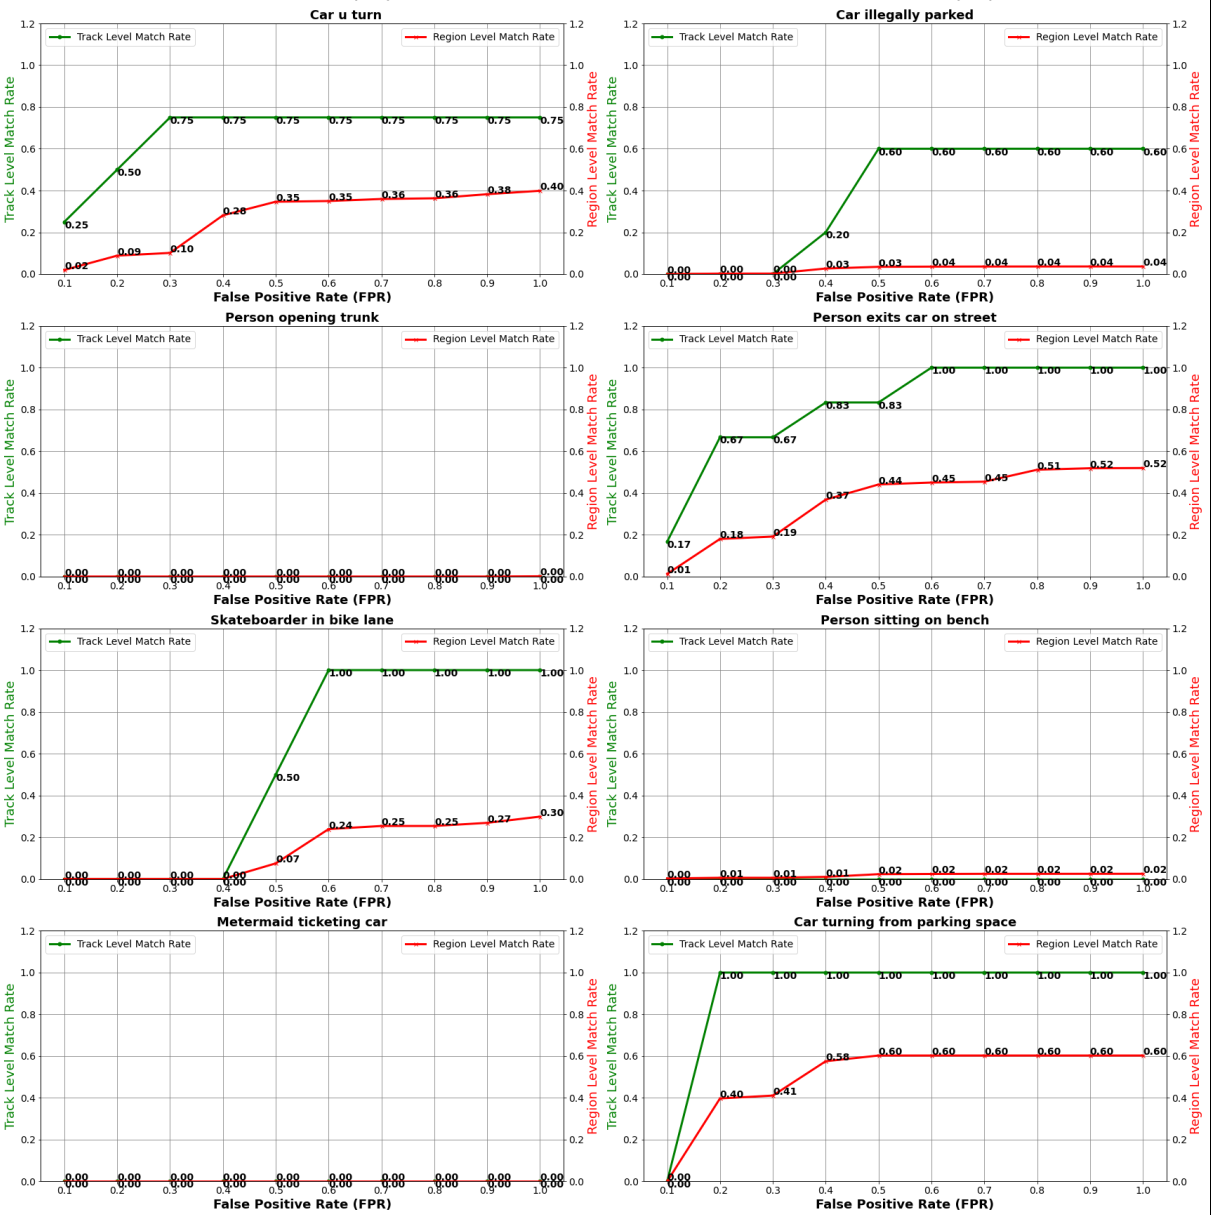}
        
    \end{subfigure}
    \hfill
    \begin{subfigure}[b]{1\textwidth}  % Width of the second figure
        \centering
        \includegraphics[width=\textwidth]{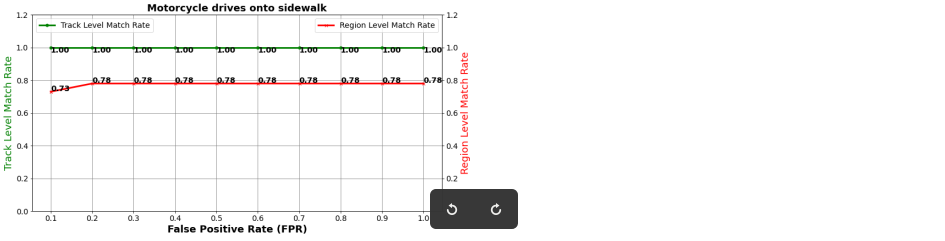}
    \end{subfigure}
    \caption{Detailed RBDC/TBDC ROC curve of our method in Street Scene Dataset. (\textbf{continued})}
    \label{fig:mainfig2}
\end{figure*}
\begin{figure}
   \centering
   \includegraphics[width=1\linewidth]{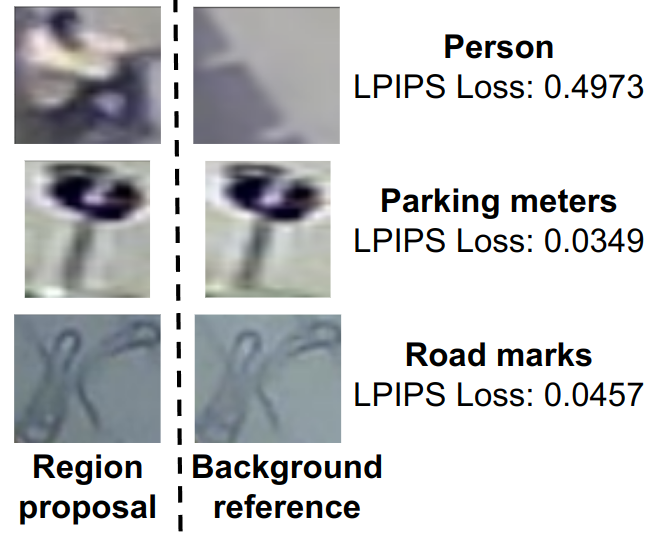}
   \caption{An example of LPIPS suppressing false detected regions.}
   \label{fig:lpips}
\end{figure}
\section{Additional Implementation Details}
Due to the page limitation, we provide further details of datasets and experiments. The detection confidence is set to 0.35 to filter out low-confidence detection results. We use Alexnet weight to calculate LPIPS loss \cite{zhang_unreasonable_2018}. To better filter false detection while keeping stationary anomalous object (e.g. person sitting on bench over the video), we choose the most similar background from training data as the reference to filter false detection. The selected background is calibrated using SIFT \cite{lowe2004distinctive} with 2000 features points. The $\sigma$ of gaussian smoothing filter is set to 7 across different dataset.

\noindent\textbf{Object detection fusion.}  For foreground subtraction, we apply a Gaussian filter to smooth the foreground mask with $\sigma =5$ and set the pixel threshold to 20. Then we find the connected components from the foreground mask and form bounding boxes around each foreground blob. We discard any box that is smaller than 15$\times$15. We use intersection-over-union (IOU) to calculate the overlap between the boxes from background subtraction and object detection. We set the IOU threshold to 0.2 to discard any duplication caused by background subtraction.
\noindent\textbf{Appearance features.} Each detected box is re-scaled to 224$\times$224$\times$3 before feeding into the CLIP vision encoder to get the CLS token. \\

\subsection{LPIPS filtering}
Compared to widely adopted benchmark datasets like UCSD ped2 and ShanghaiTech, detecting objects in Street Scene \cite{ramachandra_street_2020} is much more challenging due to the perspective and various lighting condition. We fuse object detection with background subtraction bounding boxes to capture both static/moving objects in the scene. Although it capture most of the objects, a large amount of false detection also introduce a significant amount of noise. 
An example is shown in Fig.~\ref{fig:lpips}. Detection model tends to detect such region and classify parking meters as person and road marks as bicycle. By utilizing extracted background image and LPIPS loss mentioned, we can reduce a significant amount of false detection.

\subsection{Datasets}
\noindent\textbf{UCSDPed2.} The UCSDPed2 Dataset \cite{weixin_li_anomaly_2014} contains 16 training and 12 testing videos under the single-scene setting with $240\times360$ resolution. The training and testing videos contain 2,550 and 2010 frames respectively. The normal videos only contains pedestrians walking on the sidewalk while the anomalies include non-pedestrians like skaters, cyclists or golf carts.

\noindent\textbf{ShanghaiTech.} The ShanghaiTech dataset \cite{liu_future_2018} contains 330 training and 107 testing videos under the multiple-scene setting with $480\times 856$ resolution. The training and testing videos contain 255,899 and 40,791 frames respectively. The normal videos only contains pedestrians walking on the sidewalk while the anomalies are mainly sudden motions like a person running or previously unseen objects like cyclists.\\ 
\section{Toy experiment}
\begin{figure}[htbp]
    \centering
    \includegraphics[width=1\linewidth]{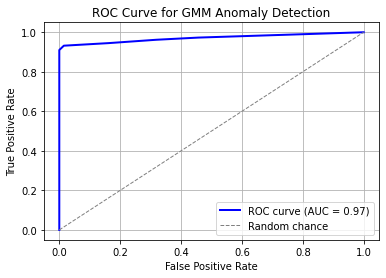}
    \caption{AUROC curve for toy experiment.}
    \label{fig:toy_result}
\end{figure}
As an abstraction of spatial context modeling, we show using a simple Gaussian Mixture Model can achieve almost perfect anomaly detection perform in the toy experiment. We provide details about setting up the toy experiment below.

We create four unique regions namely "park lane", "drive way", "bicycle lane" and "park lane". We further pre-define a set of normalcy rules like person only appears on walkway shown in \ref{alg:toy}. Then we generate 10000 samples using the normalcy rule. As for evaluation, we randomly generate 10000 samples for both normal and abnormal events. We use BIC search to train a Gaussian Mixture Model with training data and evaluate the performance on the testing data. We use AUC as the evaluation metric and the result is shown in Fig.~\ref{fig:toy_result}.

\begin{lstlisting}[style=jupyterpython, caption={Normalcy rules for creating synthetic dataset.}]
# Define variables
variables = {
    'Region': ['walkway', 'bicycle lane', 'car lane', 'park lane'],
    'Object': ['car', 'person', 'cyclist'],
    'Speed': ['fast', 'medium', 'slow']
}

# Define joint probability hints for Region-Object and Object-Speed
joint_probability_hints = {
    ('walkway', 'person'): 1.0,  # Pedestrian only shows at walkways
    ('bicycle lane', 'cyclist'): 1.0,  # Cyclist only shows at bike lanes
    ('car lane', 'car'): 0.8,  # Cars mostly in car lanes
    ('park lane', 'person'): 0.3  # Persons can be in park lanes with some probability
}

# Define joint probability hints for Object-Speed
object_speed_hints = {
    ('car', 'fast'): 0.8,  # Cars are mostly fast
    ('person', 'slow'): 0.7,  # Persons are mostly slow
    ('cyclist', 'medium'): 0.9  # Cyclists are mostly medium speed
}

# Define constraints for Region-Object and Object-Speed
constraints = {
    ('walkway', 'car'): 0.0,  # Cars should not appear in walkways
    ('bicycle lane', 'car'): 0.0,  # Cars should not appear in bike lanes
    ('car lane', 'person'): 0.0,  # Persons should not appear in car lanes
    ('park lane', 'cyclist'): 0.0,  # Cyclists should not appear in park lanes
}

object_speed_constraints = {
    ('car', 'slow'): 0.0,  # Cars should not be slow
    ('person', 'fast'): 0.0,  # Persons should not be fast
    ('cyclist', 'fast'): 0.1  # Cyclists should not be fast
}

# Define default probabilities for each variable
default_probabilities = {
    'Region': [0.25, 0.25, 0.25, 0.25],  # Probability for regions
    'Object': [0.33, 0.33, 0.34],  # Probability for objects initially
    'Speed': [0.3, 0.5, 0.2]  # Speeds as per initial probability
}
\end{lstlisting}
\label{alg:toy}

\bibliographystyle{ieee_fullname}
\bibliography{submitbib}
